# Supplementary material for: CUNI Submission in WMT22 General Task
Source: arXiv:2211.16174 source file (2022-11-29)
Supplement: Supplementary file 1 [file appendixA.tex]

\section{Appendix A}
\begin{figure*}[]

\includegraphics[width=1.00\textwidth]{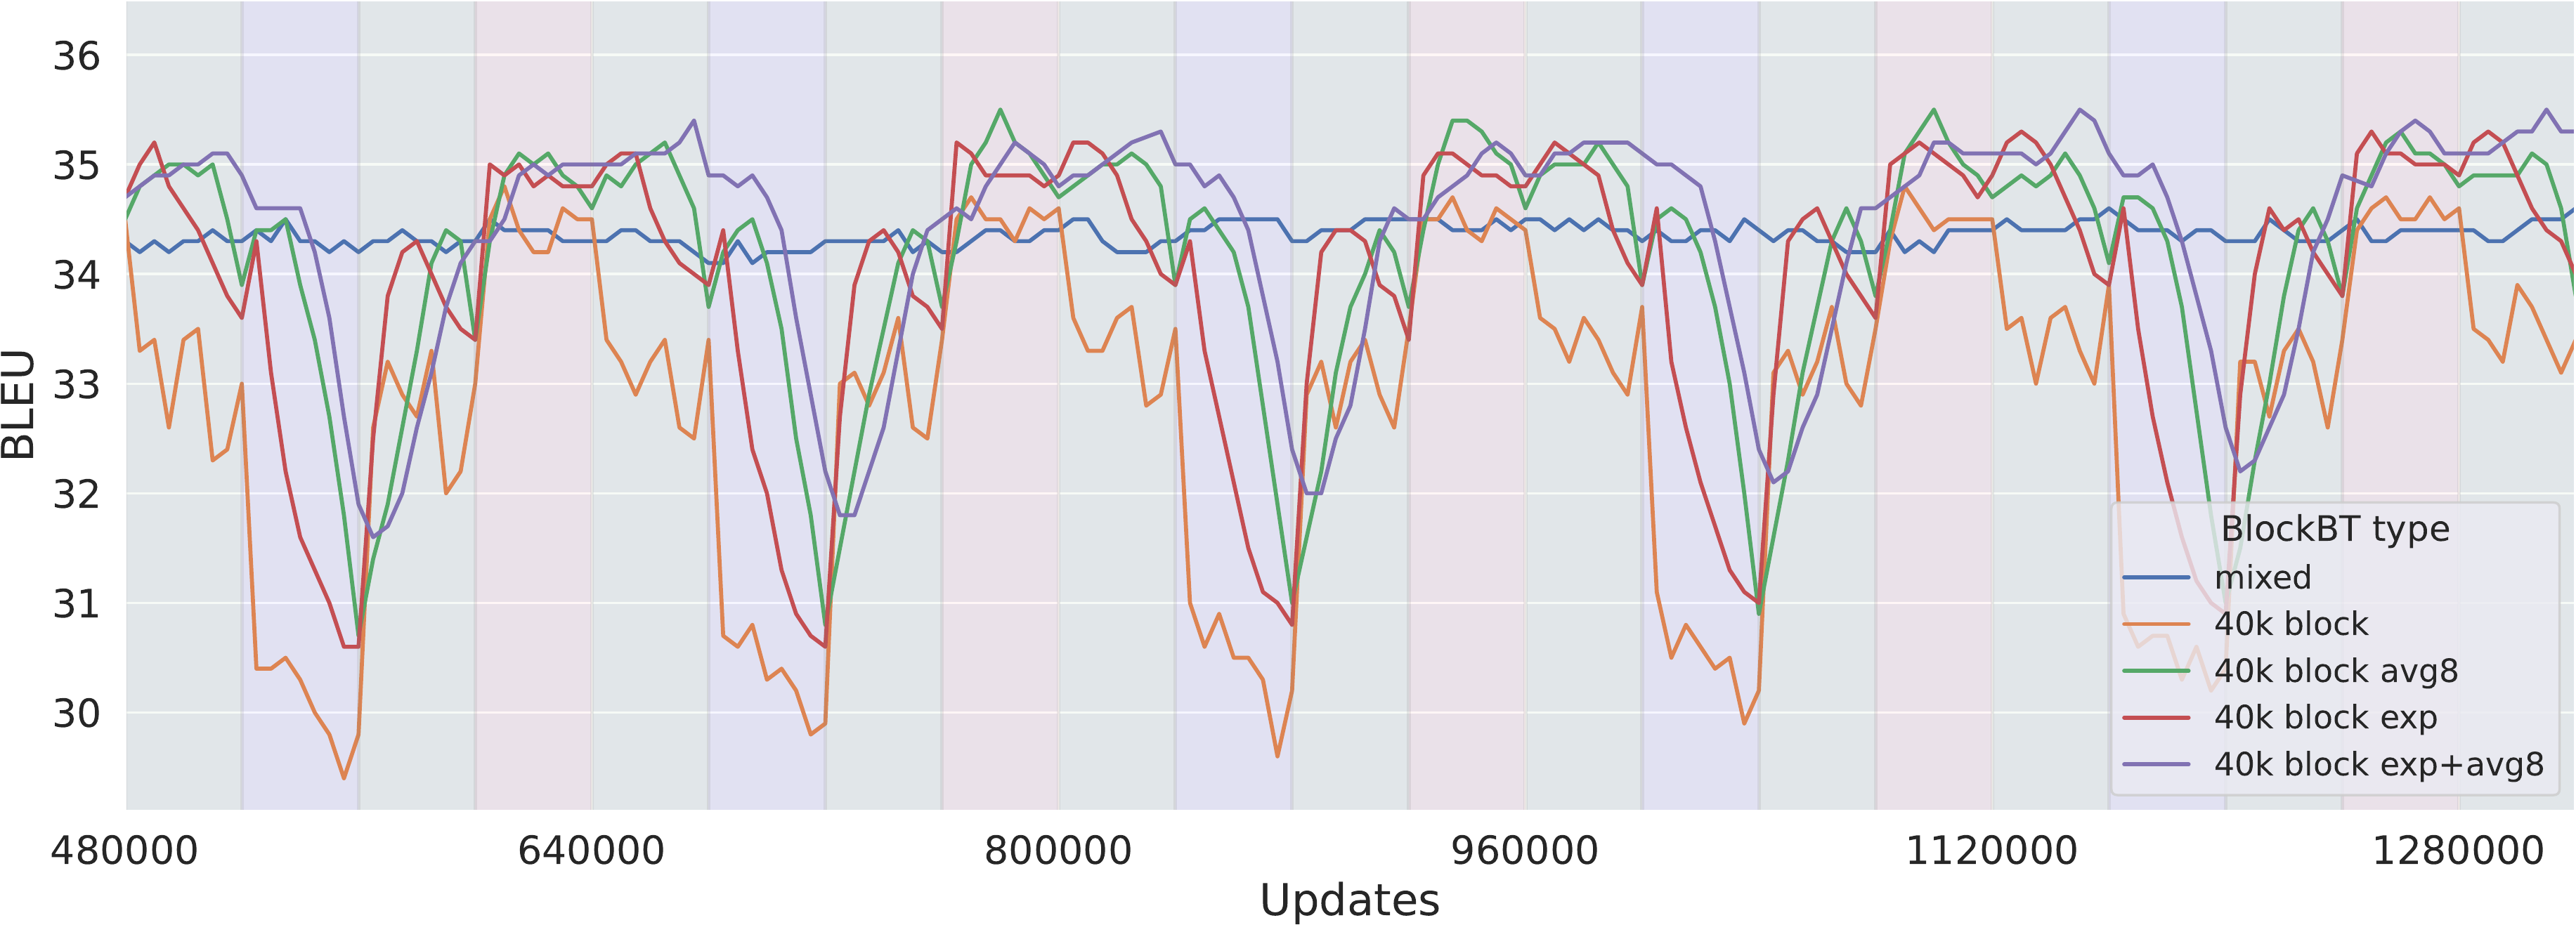}
\hspace*{-5pt}\includegraphics[width=1.00\textwidth]{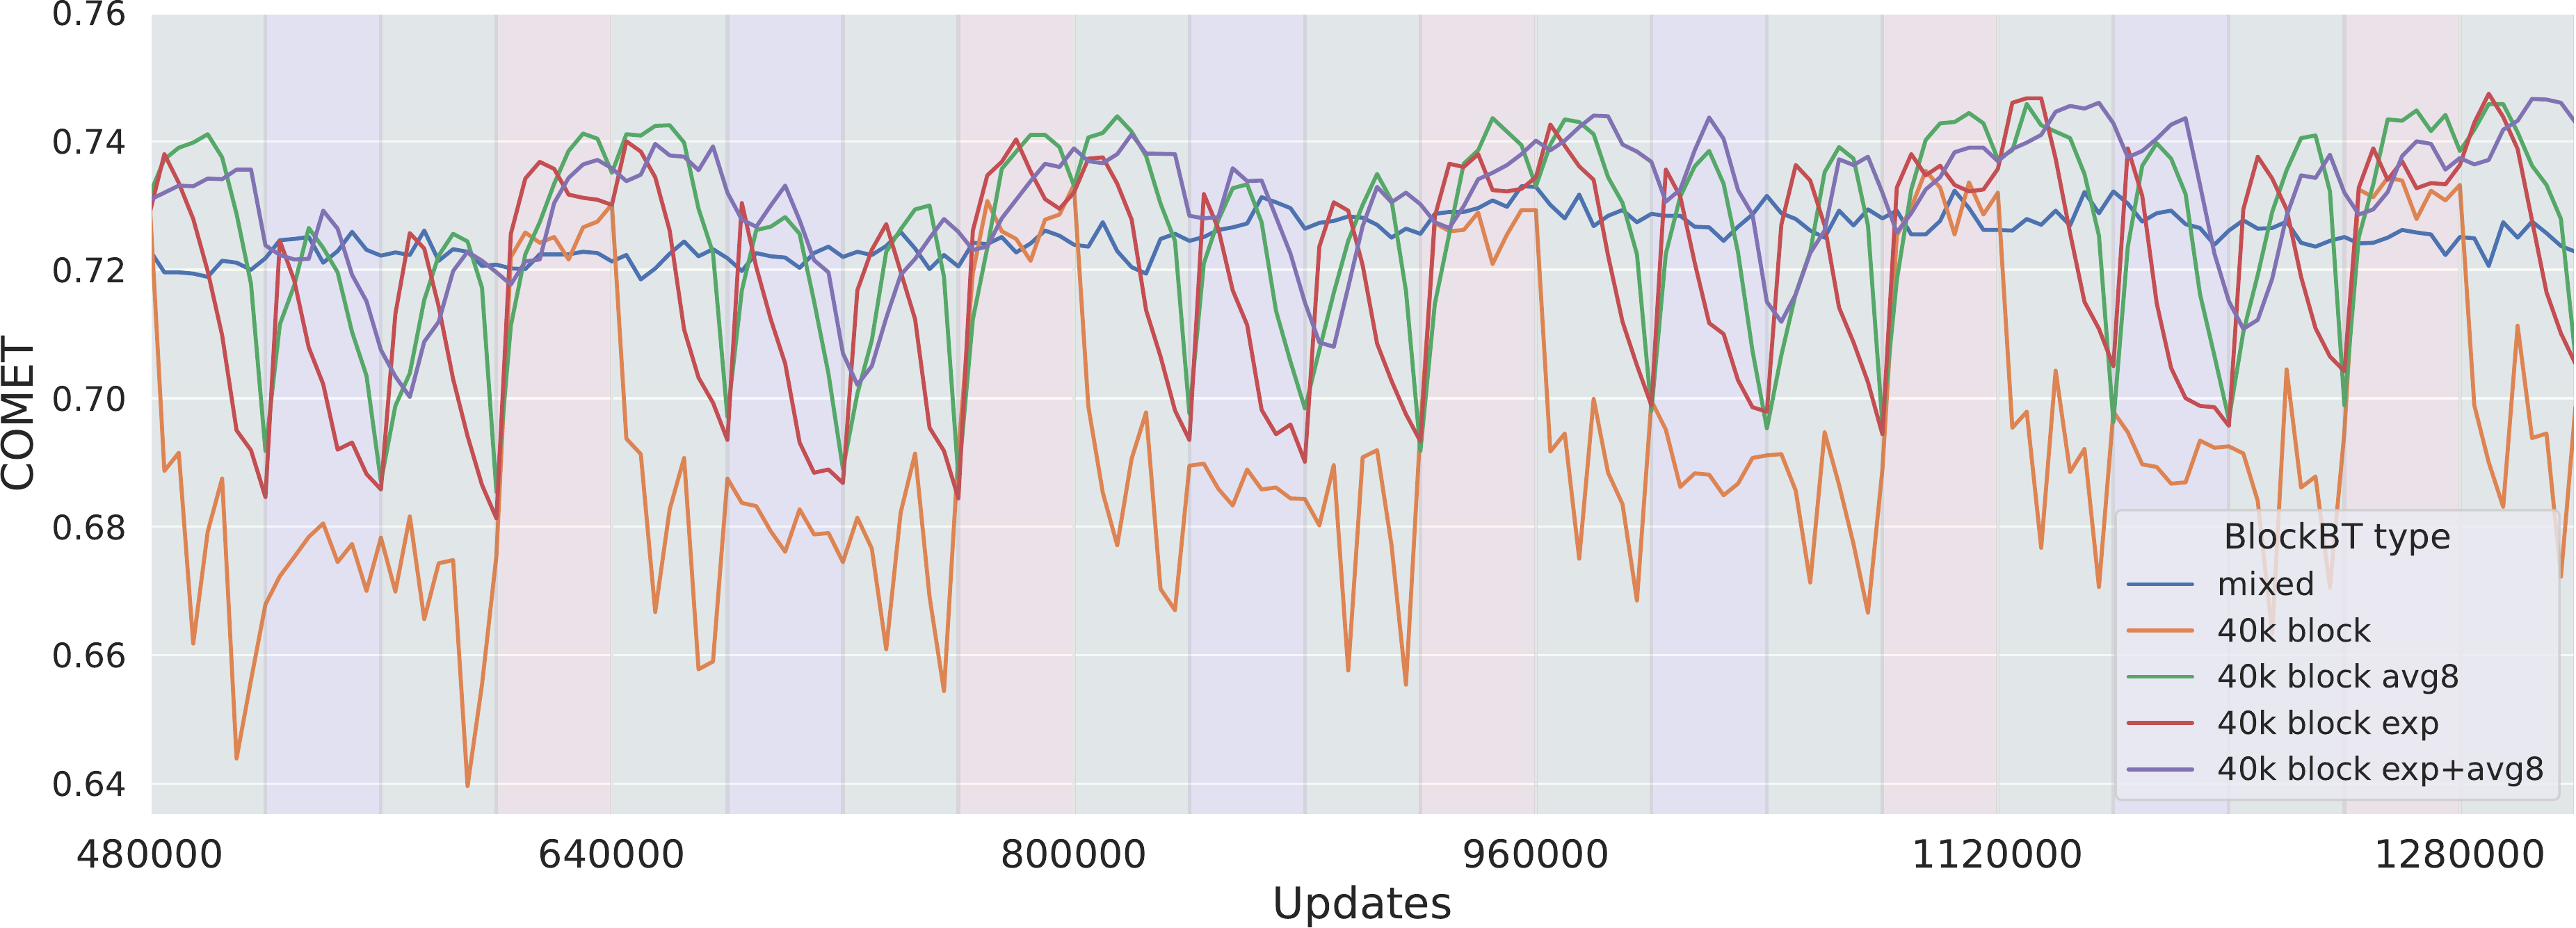}
\caption{Comparison of different training regimes for EN-CS translation on newstest20 in terms of BLEU (top) and COMET (bottom). Background colors for block-BT regime show which part of training data was used for given part of the training. Green means authentic parallel data, blue is CS->EN backtranslation and red is EN->CS forward translation.}
\label{fig:mixed_avg_exp}
\end{figure*}
